# Supplementary material for: Resolving Discrepancies in Calculations of Mechanical Properties of CH\textsubscript{3}NH\textsubscript{3}PbI\textsubscript{3} Perovskites
Source: arXiv:2412.17771 ancillary file (2024-12-23)
Supplement: Supplementary file 1 [file supplementary.pdf]

# Supplementary Information: Resolving Discrepancies in Mechanical Properties of $CH_3NH_3PbI_3$ Perovskites

Kuntal Talit[1,2] and David A. Strubbe[2*]

[1] *Department of Materials Science and Engineering, University of California, Merced, CA 95343 and*

[2] *Department of Physics, University of California, Merced, CA 95343*

## I. FORMULAE USED IN THE CALCULATION OF POLYCRYSTALLINE AVERAGES

**Voigt approximation:** [1]

$$K_V = \frac{1}{9}(C_{11} + C_{22} + C_{33}) + \frac{2}{9}(C_{12} + C_{13} + C_{23}) \tag{1}$$

$$G_V = \frac{1}{15}(C_{11} + C_{22} + C_{33} - C_{12} - C_{13} - C_{23}) + \frac{1}{5}(C_{44} + C_{55} + C_{66}) \tag{2}$$

$$\nu_V = \frac{3K_V - 2G_V}{6K_V + 2G_V} \tag{3}$$

$$E_V = \frac{9K_V G_V}{3K_V + G_V} \tag{4}$$

**Reuss approximation:** [1]

$$K_R = \frac{1}{(S_{11} + S_{22} + S_{33}) + 2(S_{12} + S_{23} + S_{13})} \tag{5}$$

$$G_R = \frac{15}{4(S_{11} + S_{22} + S_{33}) - 4(S_{12} + S_{23} + S_{13}) + 3(S_{44} + S_{55} + S_{66})} \tag{6}$$

$$\nu_R = \frac{3K_R - 2G_R}{6K_R + 2G_R} \tag{7}$$

$$E_R = \frac{9K_R G_R}{3K_R + G_R} \tag{8}$$

**Hill approximation:** [1]

$$G_H = \frac{1}{2}(G_V + G_R) \tag{9}$$

$$K_H = \frac{1}{2}(K_V + K_R) \tag{10}$$

$$E_H = \frac{9K_H G_H}{3K_H + G_H} \tag{11}$$

**Universal anisotropic index:** [2]

$$A^U = 5\frac{G_V}{G_R} + \frac{K_V}{K_R} - 6 \geq 0 \tag{12}$$

* dstrubbe@ucmerced.edu

## II. STRUCTURE INFORMATION: QUANTUM ESPRESSO INPUT FILES

### A. Orthorhombic MAPI

```
&CONTROL
  calculation='scf',
  outdir='.',
  prefix='pvsk_otrho',
  pseudo_dir='../Pseudopotential/NC.SR.ONCVPSP_V0.4_LDA',
  etot_conv_thr=1.0D-9,
  forc_conv_thr=1.0D-8,
  verbosity='high',
  nstep=1000,
/

&SYSTEM
  ibrav=0,
  celldm(1)=15.7870744008d0,
  nat=48,
  ntyp=5,
  ecutwfc=80,
/

&ELECTRONS
  conv_thr=1d-10,
  mixing_beta=0.7d0,
/

ATOMIC_SPECIES
  C 12.010700d0 C.upf
  H 1.007940d0 H.upf
  I 126.904000d0 I.upf
  N 14.006700d0 N.upf
  Pb 207.200000d0 Pb.upf

ATOMIC_POSITIONS (crystal)
C        0.509517458   0.250000000   0.945182641
C        0.490482542   0.750000000   0.054817359
C        0.990482542   0.750000000   0.445182641
C        0.009517458   0.250000000   0.554817359
N        0.434678540   0.250000000   0.096212921
N        0.565321460   0.750000000   0.903787079
N        0.065321460   0.750000000   0.596212921
N        0.934678540   0.250000000   0.403787079
H        0.471758366   0.317792720   0.156821682
H        0.528241634   0.682207280   0.843178318
H        0.028241634   0.682207280   0.656821682
H        0.971758366   0.317792720   0.343178318
H        0.528241634   0.817792720   0.843178318
H        0.471758366   0.182207280   0.156821682
H        0.971758366   0.182207280   0.343178318
H        0.028241634   0.817792720   0.656821682
H        0.307063275   0.250000000   0.088019327
H        0.692936725   0.750000000   0.911980673
H        0.192936725   0.750000000   0.588019327
H        0.807063275   0.250000000   0.411980673
H        0.470051404   0.322315598   0.883844311
H        0.529948596   0.677684402   0.116155689
```

```
H        0.029948596   0.677684402   0.383844311
H        0.970051404   0.322315598   0.616156689
H        0.529948596   0.822315598   0.116155689
H        0.470051404   0.177684402   0.883844311
H        0.970051404   0.177684402   0.616156689
H        0.029948596   0.822315598   0.383844311
H        0.643326673   0.250000000   0.957137160
H        0.356673327   0.750000000   0.042862840
H        0.856673327   0.750000000   0.457137160
H        0.143326673   0.250000000   0.542862840
Pb       0.500000000   0.000000000   0.500000000
Pb       0.000000000   0.000000000   0.000000000
Pb       0.500000000   0.500000000   0.500000000
Pb       0.000000000   0.500000000   0.000000000
I        0.525134442   0.250000000   0.528986214
I        0.474865558   0.750000000   0.471013786
I        0.974865558   0.750000000   0.028986214
I        0.025134442   0.250000000   0.971013786
I        0.820192693   0.970335227   0.689507387
I        0.179807307   0.029664773   0.310492613
I        0.679807307   0.029664773   0.189507387
I        0.320192693   0.970335227   0.810492613
I        0.179807307   0.470335227   0.310492613
I        0.820192693   0.529664773   0.689507387
I        0.320192693   0.529664773   0.810492613
I        0.679807307   0.470335227   0.189507387

K_POINTS {automatic}
  5 4 5  1 1 1

CELL_PARAMETERS (alat= 15.78707440)
   0.980420667   0.000000000   0.000000000
   0.000000000   1.491920841   0.000000000
   0.000000000   0.000000000   1.058276350
```

### B. Tetragonal (I4cm) MAPI

```
&CONTROL
  calculation='scf',
  outdir='.',
  prefix='tetragonal',
  pseudo_dir='../Pseudopotential/NC.SR.ONCVPSP_V0.4_LDA',
  etot_conv_thr=1.0D-9,
  forc_conv_thr=1.0D-8,
  nstep=10000,
  verbosity='low',
/

&SYSTEM
  ibrav=0,
  celldm(1)=16.4316599819d0,
  nat=48,
  ntyp=5,
  ecutwfc=80,
/

&ELECTRONS
```

```
  conv_thr=1d-10,
  mixing_beta=0.7d0,
/

ATOMIC_SPECIES
  C 12.010700d0 C.upf
  H 1.007940d0 H.upf
  I 126.904000d0 I.upf
  N 14.006700d0 N.upf
  Pb 207.200000d0 Pb.upf

ATOMIC_POSITIONS (crystal)
C        0.028975534   0.500796712   0.249292862
C        0.536063304   0.043885171   0.247443711
C        0.043862358   0.536134568   0.747400854
C        0.500795660   0.028933460   0.749328121
N        0.922539300   0.611362428   0.196294988
N        0.426905680   0.931390920   0.199888773
N        0.931401426   0.426918517   0.699871295
N        0.611387713   0.922528506   0.696316058
H        0.656320145   0.016347028   0.221242957
H        0.528255634   0.035571142   0.334259146
H        0.504722354   0.163162681   0.221184489
H        0.452110444   0.815461964   0.221966802
H        0.432650745   0.936583096   0.117423990
H        0.310133610   0.954450153   0.221084493
H        0.930227417   0.600033139   0.114220567
H        0.948999159   0.728228380   0.214619640
H        0.805074045   0.591055376   0.217229820
H        0.150307309   0.524926832   0.223849927
H        0.997285222   0.380142993   0.227081665
H        0.018440833   0.514886780   0.335585247
H        0.954463758   0.310168682   0.721113339
H        0.936631635   0.432584369   0.617405306
H        0.815459742   0.452129617   0.721923434
H        0.163155224   0.504786240   0.721169642
H        0.035516853   0.528405893   0.834218020
H        0.016318631   0.656362475   0.721149773
H        0.728244204   0.948968204   0.714678354
H        0.600117387   0.930282489   0.614241754
H        0.591059015   0.805050477   0.717202943
H        0.524964510   0.150284524   0.723950145
H        0.514817016   0.018318664   0.835620305
H        0.380155272   0.997281829   0.727062631
Pb       0.509483519   0.513945681   0.988568614
Pb       0.513937112   0.509463664   0.488568721
Pb       0.029281973   0.011051060   0.490216139
Pb       0.011075505   0.029293484   0.990216435
I        0.697940514   0.834399451   0.994920045
I        0.333252927   0.198560688   0.996934324
I        0.202813795   0.714353130   1.002368409
I        0.839417192   0.351903222   0.986264084
I        0.351885315   0.839386086   0.486303428
I        0.714336255   0.202785648   0.502384479
I        0.834389572   0.697920711   0.494903449
I        0.198547662   0.333234603   0.496899132
I        0.520646986   0.524765167   0.239976981
I        0.524762615   0.520638083   0.739975343
```

```
I        0.013998162   0.018889645   0.742089276
I        0.018867754   0.013982374   0.242088085

K_POINTS {automatic}
  5 5 4 1 1 1

CELL_PARAMETERS (alat= 16.43165998)
   0.979807479   0.000365594  -0.002594346
   0.001128900   0.979811798  -0.001516903
   0.008879481   0.007174722   1.451802233
```

### C. Tetragonal (I4/mcm) MAPI

```
&CONTROL
  calculation='scf',
  outdir='.',
  prefix='I4mcm_merced',
  pseudo_dir='./LDA',
  etot_conv_thr=1.0D-9,
  forc_conv_thr=1.0D-8,
  verbosity='high',
  nstep=1000,
/

&SYSTEM
  ibrav=0,
  celldm(1)=16.9119338764d0,
  nat=48,
  ntyp=5,
  ecutwfc=80,
/

&ELECTRONS
  conv_thr=1d-10,
  mixing_beta=0.7d0,
/

ATOMIC_SPECIES
  C 12.010700d0 C.upf
  H 1.007940d0 H.upf
  I 126.904000d0 I.upf
  N 14.006700d0 N.upf
  Pb 207.200000d0 Pb.upf

ATOMIC_POSITIONS (crystal)
N            0.9067084507        0.5963654811        0.2174935726
N            0.9067090441        0.4036338027        0.7174952812
N            0.5932901660        0.0963661947        0.2174944797
N            0.5932914023        0.9036348593        0.7174946488
C            0.0168580176        0.4901817484        0.2707744800
C            0.0168590746        0.5098172418        0.7707749254
C            0.4831413399        0.9901813314        0.2707747144
C            0.4831415565        0.0098178408        0.7707740213
H            0.1370755001        0.5200900600        0.2465642353
H            0.0044659261        0.5029317037        0.3570810249
H           -0.0090443289        0.3683962012        0.2474621377
H            0.7902123158        0.5719310165        0.2378791806
```

```
H             0.9290396011        0.7141947712        0.2361371662
H             0.9156415332        0.5857832231        0.1354059756
H             0.1370764242        0.4799103082        0.7465636692
H            -0.0090449048        0.6316024669        0.7474612749
H             0.0044669500        0.4970642623        0.8570814671
H             0.7902127422        0.4280679039        0.7378807446
H             0.9156423842        0.4142165119        0.6354077927
H             0.9290398516        0.2858043891        0.7361393276
H             0.3629241454        1.0200898781        0.2465637001
H             0.5090443966        0.8683960879        0.2474616872
H             0.4955345573        0.0029324919        0.3570811556
H             0.7097862271        0.0719312043        0.2378797848
H             0.5843555581        0.0857845151        0.1354070431
H             0.5709590720        0.2141953317        0.2361384413
H             0.3629237397       -0.0200904938        0.7465639449
H             0.4955352645        0.9970656873        0.8570802879
H             0.5090450126        0.1316032609        0.7474605408
H             0.7097879544        0.9280698882        0.7378798090
H             0.5709594852        0.7858051990        0.7361379693
H             0.5843568584        0.9142193051        0.6354074011
Pb            0.0088496793        0.0107390236        0.0100531223
Pb            0.0088508902        0.9892599579        0.5100529300
Pb            0.4911489253        0.4892600777        0.5100518177
Pb            0.4911495382        0.5107395403        0.0100528250
I             0.1763874538        0.6880541264        0.0175115323
I             0.8113766029        0.3229015406        0.0153775678
I             0.3236115716        0.1880535917        0.0175118896
I             0.6886252560        0.8229008651        0.0153785878
I             0.6886226319        0.1770980310        0.5153808240
I             0.3236140861        0.8119477032        0.5175118194
I             0.8113783693        0.6770966841        0.5153809398
I             0.1763860412        0.3119477891        0.5175110478
I             0.9941951667        0.9997127488        0.2615205466
I             0.9941906896        0.0002890804        0.7615207823
I             0.5058114159        0.5002881571        0.7615203246
I             0.5058063673        0.4997154089        0.2615195561


K_POINTS {automatic}
  5 4 5 1 1 1

CELL_PARAMETERS (alat= 16.91193388)
   0.953957482  -0.000017614  -0.000004625
   0.000016632   0.951906889   0.000014049
   0.000003284  -0.000009893   1.410104436
```

## D. Cubic MAPI

```
&CONTROL
  calculation='scf',
  outdir='.',
  prefix='pvsk_100',
  pseudo_dir='./NC.SR.ONCVPSP_V0.4_LDA',
  etot_conv_thr=1.0D-9,
  forc_conv_thr=1.0D-8,
  nstep=10000,
/
```

```
&SYSTEM
  ibrav=0,
  celldm(1)=12.3682574853d0,
  nat=12,
  ntyp=5,
  ecutwfc=100,
/

&ELECTRONS
  conv_thr=1d-10,
  mixing_beta=0.7d0,
/


ATOMIC_SPECIES
  C 12.010700d0 C.upf
  H 1.007940d0 H.upf
  I 126.904000d0 I.upf
  N 14.006700d0 N.upf
  Pb 207.200000d0 Pb.upf

ATOMIC_POSITIONS (crystal)
C        0.891791779  -0.000021128   0.457639650
N        0.108995215  -0.000018881   0.550427677
H        0.908911248  -0.000019639   0.282551212
H        0.803815280   0.147550763   0.510774245
H        0.803808981   0.852403269   0.510775694
H        0.198705830   0.138312688   0.504194084
H        0.198693773   0.861641983   0.504213935
H        0.105216403  -0.000011816   0.716847054
Pb       0.444621483   0.499958675   0.975838514
I        0.417671992   0.500004750   0.473538440
I        0.397876044  -0.000032639   0.030817505
I        0.935670681   0.499997866   0.909512158

K_POINTS {automatic}
  6 6 6 1 1 1

CELL_PARAMETERS (alat= 12.36825749)
   0.941669545  -0.000133982  -0.000482895
   0.000098601   0.934259294   0.000033225
   0.020320700  -0.000023095   0.957261222
```


[1] R. Hill, Proc. Phys. Soc. A **65**, 349 (1952).
[2] S. I. Ranganathan and M. Ostoja-Starzewski, Phys. Rev. Lett. **101**, 055504 (2008).
